# Supplementary material for: Gaussianization Flows
Source: arXiv:2003.01941 source file (2020-03-04)
Supplement: Supplementary file 2 [file appendix_old.tex]

\onecolumn
\section{Proofs}
\begin{lemma}\label{lem:1}
Let $\bfx \in \mbb{R}^2$ be a random vector with a continuously differentiable probability density function $p(x_1, x_2)$ with the following properties:
\begin{enumerate}
    \item For any rotation matrix $R\in \mbb{R}^{2\times 2}$, $R \bfx$ has the same distribution as $\bfx$;
    \item For $i=1, 2$, $p(x_i) = \frac{1}{\sqrt{2\pi}}e^{-\frac{x_i^2}{2}}$.
\end{enumerate}
Then $p(x_1, x_2) = p(x_1) p(x_2) = \frac{1}{2\pi}e^{-\frac{x_1^2 + x_2^2}{2}}$.
\end{lemma}
\begin{proof}
Property~1 implies that $p(x_1, x_2)$ is rotational invariant. So there exists a function $\phi: \mbb{R} \to \mbb{R}$ such that
\begin{align*}
    p(x_1, x_2) = \phi(x_1 ^ 2 + x_2 ^2) = \phi(r^2)
\end{align*}
From property~2, we have
\begin{align}
    \int_{-\infty}^{\infty} \phi(x_1^2 +  x_2^2) \ud x_2 = \frac{1}{\sqrt{2\pi}} e^{-\frac{x_1^2}{2}} \label{eqn:marginal}
\end{align}
Taking the derivative \wrt $x_1$ for both sides of \eqnref{eqn:marginal}, we obtain
\begin{align}
2 \int_{-\infty}^{\infty} \phi'(r^2) x_1 \ud x_2 = - x_1 \frac{1}{\sqrt{2\pi}}  e^{-\frac{x_1^2}{2}} \label{eqn:grad}
\end{align}
Comparing \eqnref{eqn:marginal} and \eqnref{eqn:grad}, we have 
\begin{align}
    \forall x_1 \in \mbb{R}: \quad \int_{-\infty}^{\infty} \phi(r^2) + 2\phi'(r^2) \ud x_2 = 0 \label{eqn:integral_equation}
\end{align}
Next, we will show that \eqnref{eqn:integral_equation} implies that $\phi(r^2) + 2\phi'(r^2) \equiv 0$. Assuming this does not hold, there exists $r_0$ such that $\phi(r_0^2) + 2\phi'(r_0^2) > 0$. Because \eqnref{eqn:integral_equation} holds for all $x_1$, we can let $x_1^2 = r_0^2$ and $x_1^2 = r_0^2 + \epsilon^2$ respectively to get
\begin{align}
    \int_{-\infty}^{\infty} \phi(r_0^2 + x_2^2) + 2\phi'(r_0^2 + x_2^2) \ud x_2 &= 0 \label{eqn:eq1}\\
    \int_{-\infty}^{\infty} \phi(r_0^2 + \epsilon^2 + x_2^2) + 2\phi'(r_0^2 +\epsilon^2 + x_2^2) \ud x_2 &= 0 \label{eqn:eq2},
\end{align}
where $\epsilon > 0$ is a small constant. Now we change variable $x_2^2 + \epsilon^2$ to $y_2^2$ in \eqnref{eqn:eq2} to get
\begin{align*}
    &\int_{-\infty}^{\infty} \phi(r_0^2 + \epsilon^2 + x_2^2) + 2\phi'(r_0^2 +\epsilon^2 + x_2^2) \ud x_2\\
    =& 2\int_{0}^{\infty} \phi(r_0^2 + \epsilon^2 + x_2^2) + 2\phi'(r_0^2 +\epsilon^2 + x_2^2) \ud x_2\\
    =& 2 \int_{\epsilon}^{\infty}[\phi(r_0^2 + y_2^2) + 2\phi'(r_0^2 + y_2^2)] \frac{y_2}{\sqrt{y_2^2 - \epsilon^2}} \ud y_2
\end{align*}
Therefore, \eqnref{eqn:eq1} - \eqnref{eqn:eq2} is
\begin{gather}
    2 \int_{0}^{\epsilon}[\phi(r_0^2 + x_2^2) + 2\phi'(r_0^2 + x_2^2)] \ud x_2 \label{eqn:term1}\\
    + 2 \int_{\epsilon}^{\infty} [\phi(r_0^2 + y_2^2) + 2\phi'(r_0^2 + y_2^2)]\left[1 - \frac{y_2}{\sqrt{y_2^2 - \epsilon^2}} \right] \ud y_2 \label{eqn:term2}.
\end{gather}
Next, we can further simplify \eqnref{eqn:term2} by changing $y_2^2 - \epsilon^2$ back to $x_2^2$, \ie,
\begin{align*}
   & 2 \int_{\epsilon}^{\infty} [\phi(r_0^2 + y_2^2) + 2\phi'(r_0^2 + y_2^2)]\left[1 - \frac{y_2}{\sqrt{y_2^2 - \epsilon^2}} \right] \ud y_2\\
   =& 2 \int_{0}^{\infty} [\phi(r_0^2 + \epsilon^2 + x_2^2) + 2\phi'(r_0^2 + \epsilon^2 + x_2^2)]\left[\frac{x_2}{\sqrt{x_2^2 + \epsilon^2}} - 1 \right] \ud x_2 \\
   =& 2 \int_{0}^{\infty} [\phi(r_0^2 + \epsilon^2 + x_2^2) + 2\phi'(r_0^2 + \epsilon^2 + x_2^2)]\left[-\frac{\epsilon^2}{2x_2^2}  + O(\epsilon^4)\right] \ud x_2\\
   =& O(\epsilon^2).
\end{align*}
Because $\phi(r_0^2) + 2\phi'(r_0^2) > 0$, and $\phi(r^2) + 2\phi'(r^2)$ is continuous, there exists $\delta > 0$ such that $\phi(r_0^2 + \epsilon^2) + 2\phi'(r_0^2 + \epsilon^2) > \delta$ as long as $\epsilon > 0$ is small enough. Hence \eqnref{eqn:term1} can be bounded by
\begin{align*}
   &2 \int_{0}^{\epsilon}[\phi(r_0^2 + x_2^2) + 2\phi'(r_0^2 + x_2^2)] \ud x_2 \\
   \geq & 2 \epsilon \delta.
\end{align*}
As a result, \eqnref{eqn:eq1} - \eqnref{eqn:eq2} can be lower bounded by
\begin{align*}
    2 \epsilon \delta + O(\epsilon^2) \geq \epsilon \delta
\end{align*}
when $\epsilon$ is small enough. This contradicts the fact that \eqnref{eqn:eq1} - \eqnref{eqn:eq2} = 0. Therefore $\phi(r^2) + 2\phi'(r^2) \equiv 0$. Solving this ordinary differential equation, we obtain
\begin{align*}
    \phi(r^2) = Ce^{-\frac{r^2}{2}}.
\end{align*}
Since $\phi(r^2) = p(x_1, x_2)$ is a normalized density, we have $C = \frac{1}{2\pi}$, and therefore
\begin{align*}
    p(x_1, x_2) = \phi(r^2) = \frac{1}{2\pi} e^{-\frac{r^2}{2}} = \frac{1}{2\pi} e^{-\frac{x_1^2+x_2^2}{2}}.
\end{align*}
\end{proof}

\begin{theorem}\label{thm:1}
Let $\bfx \in \mbb{R}^d$ be a random vector with a continuously differentiable probability density function $p(x_1, x_2)$ with the following properties:
\begin{enumerate}
    \item For any rotation matrix $R\in \mbb{R}^{d\times d}$, $R \bfx$ has the same distribution as $\bfx$;
    \item For $i=1, 2, \cdots, d$, $p(x_i) = \frac{1}{\sqrt{2\pi}}e^{-\frac{x_i^2}{2}}$.
\end{enumerate}
Then $\bfx \sim \mcal{N}(0, I_d)$.
\end{theorem}

\begin{proof}
We prove the statement by induction. From \lemref{lem:1} we know that the theorem holds when $d = 2$. Assume the statement holds for $d = k-1$. Now consider the case $d=k$. Since $p(x_1, x_2, \cdots, x_k)$ is rotational-invariant, we know that $p(x_1, x_2, \cdots, x_{k-1})$ is also a rotational invariant distribution with Gaussian marginals, so by our induction assumption
\begin{align}
    p(x_1, x_2, \cdots, x_{k-1}) = \frac{1}{(2\pi)^{\frac{k-1}{2}}} e^{-\frac{x_1^2 + x_2^2 + \cdots + x_{k-1}^2}{2}} = \frac{1}{(2\pi)^{\frac{k-1}{2}}} e^{-\frac{r^2}{2}}e^{\frac{x_k^2}{2}},\label{eqn:k-1}
\end{align}
where $r^2 = x_1^2 + \cdots + x_k^2$. Due to rotational invariance again, we know there exists some function $\phi: \mbb{R} \to \mbb{R}$ such that
\begin{align}
    p(x_1, x_2, \cdots, x_k) = \phi(r^2).\label{eqn:invariance}
\end{align}
Combining \eqnref{eqn:k-1} and \eqnref{eqn:invariance}, we have the following equality
\begin{align}
    \int \phi(r^2) \ud x_k = \frac{1}{(2\pi)^{\frac{k-1}{2}}} e^{-\frac{r^2}{2}}e^{\frac{x_k^2}{2}}. \label{eqn:induction}
\end{align}
Taking the derivative \wrt $x_1$ for both sides, we have
\begin{align}
    2 \int \phi'(r^2) x_1 \ud x_k = -x_1 \frac{1}{(2\pi)^{\frac{k-1}{2}}} e^{-\frac{r^2}{2}}e^{\frac{x_k^2}{2}}. \label{eqn:induction_grad}
\end{align}
Comparing \eqnref{eqn:induction} and \eqnref{eqn:induction_grad}, we have
\begin{align*}
    \forall x_1, x_2, \cdots, x_{k-1}:\quad \int \phi(r^2) + 2\phi'(r^2) \ud x_k = 0.
\end{align*}
Following a similar argument as in the proof of \lemref{lem:1}, we can conclude that $\phi(r^2) + 2\phi'(r^2) \equiv 0$. We can then solve this ordinary differential equation and get
\begin{align*}
    \phi(r^2) = C e^{-\frac{r^2}{2}}.
\end{align*}
Because $\phi(r^2)$ is a normalized distribution, $C = \frac{1}{(2\pi)^{k/2}}$. Therefore the theorem statement holds for $d=k$ as well. Thus our proof is finished by induction.
\end{proof}
\begin{theorem}
Let $\bfx \in \mbb{R}^d$ be a random vector with a continuously differentiable probability density function $p(x_1, x_2, \cdots, x_d) $. If for all rotation matrix $R \in \mbb{R}^{d\times d}$, the rotated random vector $\bfx' = R \bfx$ has a probability density function $q_R(x_1', x_2', \cdots, x_d')$ which satisfies
\begin{align*}
    \forall i = 1, 2, \cdots, d: \quad q_R(x_i') = \frac{1}{\sqrt{2\pi}}e^{-\frac{(x_i')^2}{2}},
\end{align*}
then $\forall R: q_R(x_1', x_2', \cdots, x_d') = p(x_1, x_2, \cdots, x_d)$. In other words, the distribution of $\bfx$ is rotational invariant.
\end{theorem}
\begin{proof}
Let $R_{1,2}$ be a Givens rotation matrix in the plane spanned by axes $x_1$, $x_2$. Suppose the rotation angle is $\theta$. Then
\begin{align*}
\begin{pmatrix}
x_1'\\
x_2'\\
\vdots\\
x_d'
\end{pmatrix}   = \begin{pmatrix}
\cos\theta & -\sin\theta & 0 & \cdots & 0\\
\sin\theta & \cos\theta & 0 & \cdots & 0\\
0 & 0 & 1 & \cdots & 0\\
\vdots & \vdots & \vdots & \ddots & \vdots\\
0 & 0 & 0 & \cdots & 1
\end{pmatrix}
\begin{pmatrix}
x_1 \\
x_2 \\
\vdots \\
x_d
\end{pmatrix}
\end{align*}
Using the change of variable formula, we know that 
\begin{align}
\forall x_1', x_2', \cdots, x_d', \theta:\quad q_{R_{1,2}}(x_1', x_2', x_3', \cdots, x_d') = p(x_1' \cos\theta + x_2' \sin\theta, -x_1'\sin\theta + x_2'\cos\theta, x_3, \cdots, x_d).\label{eqn:cofv}
\end{align}
From Sklar's theorem, we can write probability densities in the form of copulas:
\begin{align*}
    p(x_1, x_2, \cdots, x_d) &= c_p(\Psi(x_1), \Psi(x_2), \cdots, \Psi(x_d)) \frac{1}{(2\pi)^{d/2}}e^{-\frac{\sum_{i=1}^d x_i^2}{2}}\\
    q_{R_{1,2}}(x_1, x_2, \cdots, x_d) &= c_{q_{R_{1,2}}}(\Psi(x_1), \Psi(x_2), \cdots, \Psi(x_d)) \frac{1}{(2\pi)^{d/2}}e^{-\frac{\sum_{i=1}^d x_i^2}{2}},
\end{align*}
where $\Psi(\cdot)$ denotes the cdf function of a standard normal distribution. Using copulas, \eqnref{eqn:cofv} can be written as
\begin{gather*}
    \forall x_1', x_2', \cdots, x_d', \theta: \\
    c_{q_{R_{1,2}}}(\Psi(x_1'), \Psi(x_2'), \Psi(x_3'), \cdots, \Psi(x_d')) = c_{p}(\Psi(x_1'\cos\theta + x_2'\sin\theta), \Psi(-x_1'\sin\theta + x_2'\cos\theta), \Psi(x_3), \cdots, \Psi(x_d)).
\end{gather*}

\end{proof}

\begin{theorem}
Let $\bfx \in \mbb{R}^d$ be a random vector with a continuously differentiable probability density function. Then there exists a sequence of rotation matrices $\{R_i\}_{i=1}^n$ and element-wise functions $\{\Phi: \mbb{R}^d \to \mbb{R}^d \}_{i=1}^n$ such that the random vector $\bfz_n$ in the following form
\begin{align*}
    \bfz_n = R_n \Phi_n (R_{n-1} \Phi_{n-1}( \cdots R_1 \Phi_1(\bfx)))
\end{align*}
converges to $\mcal{N}(0, I_d)$ in probability.
\end{theorem}
\begin{proof}
In order to prove $\bfz_n \stackrel{d}{\to} \mcal{N}(0, I_d)$, we can equivalently prove $\operatorname{KL}(p(\bfz_n) \| \mcal{N}(0,I_d)) \to 0$. We first note that
\begin{align}
    \operatorname{KL}(p(\bfz_n) \| \mcal{N}(0, I_d)) = \operatorname{KL}\left(p(\bfz_n) \| \prod_{i=1}^d z_{n,i}\right) + \sum_{i=1}^d \operatorname{KL}(p(z_{n,i} \| \mcal{N}(0, 1)), \label{eqn:decomp}
\end{align}
where $z_{n,i} = (\bfz_n)_i$ is the $i$-th element of $\bfz_n$. Clearly, rotation $R_i$ does not change $\operatorname{KL}(p(\bfz_n) \| \mcal{N}(0, I_d))$, and element-wise operation $\Phi_i$ does not change the first term in \eqnref{eqn:decomp}. If we choose $\Phi_n(\bfz_{n-1}) = \Psi^{-1}(F_{\bfz_{n-1}}(\bfz_{n-1}))$, where $\Psi$ is the cdf of a standard normal distribution, the second term of \eqnref{eqn:decomp} will vanish, and we have $\operatorname{KL}(p(\bfz_n) \| \mcal{N}(0, I_d)) < \operatorname{KL}(p(\bfz_{n-1}) \| \mcal{N}(0, I_d))$. 

As long as $\operatorname{KL}(p(\bfz_n) \| \mcal{N}(0, I_d)) > 0$, there exists a rotation matrix $R_n$ such that under the optimal choice of $\Phi_{n+1}$, $\operatorname{KL}(p(\bfz_{n+1}) \| \mcal{N}(0, I_d)) < \operatorname{KL}(p(\bfz_n) \| \mcal{N}(0, I_d))$. This is because a non-Gaussian distribution cannot be rotation-invariant
\end{proof}

\section{Image reconstruction and samples}
\begin{figure}%
    \centering
    \begin{subfigure}[b]{0.3\textwidth}
        \includegraphics[width=\textwidth]{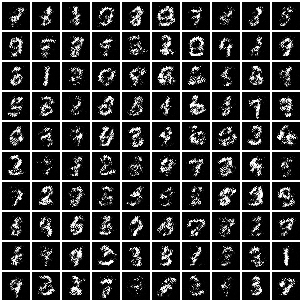}
    \end{subfigure}
    \begin{subfigure}[b]{0.3\textwidth}
        \includegraphics[width=\textwidth]{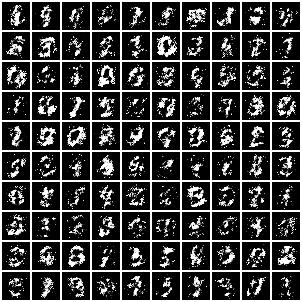}
    \end{subfigure}
    \begin{subfigure}[b]{0.3\textwidth}
        \includegraphics[width=\textwidth]{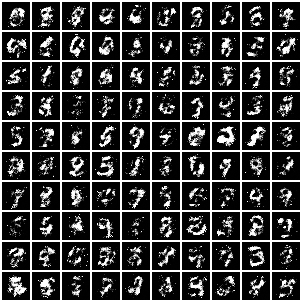}
    \end{subfigure}
    \caption{\textbf{Left:} MADE MNIST samples. \textbf{Middle:} Iterative Gaussiainzation MNIST samples. \textbf{Right:}
    Gaussianization flow MNIST samples.}
    \label{fig:mnist_samples}
\end{figure}

\begin{figure}%
    \centering
    \begin{subfigure}[b]{0.3\textwidth}
        \includegraphics[width=\textwidth]{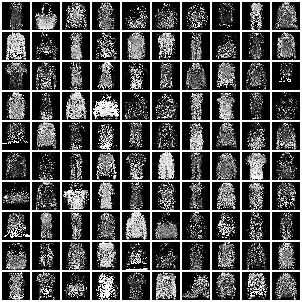}
    \end{subfigure}
    \begin{subfigure}[b]{0.3\textwidth}
        \includegraphics[width=\textwidth]{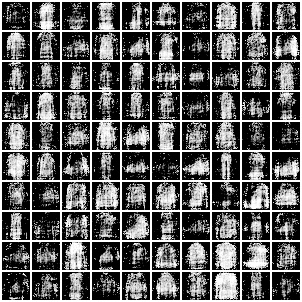}
    \end{subfigure}
    \begin{subfigure}[b]{0.3\textwidth}
        \includegraphics[width=\textwidth]{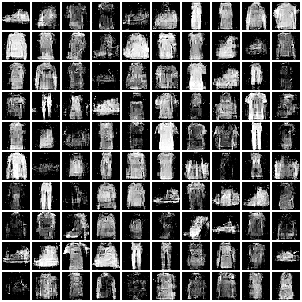}
    \end{subfigure}
    \caption{\textbf{Left:} MADE Fashion MNIST samples.
    \textbf{Middle:} Iterative Gaussiainzation Fashion MNIST samples.\textbf{Right:}
    Gaussianization flow Fashion MNIST samples.}
    \label{fig:fmnist_samples}
\end{figure}
